# Supplementary material for: Conjoining uncooperative societies facilitates evolution of cooperation
Source: arXiv:1805.12215 source file (2018-06-14)
Supplement: Supplementary file 1 [file SI_Naghmeh__2_.pdf]

| Graph                               | $\left(\frac{b}{c}\right)^*$ |
|-------------------------------------|------------------------------|
| Star                                | Inf                          |
| Star of Stars                       | 2                            |
| Two Stars                           | $\frac{5}{2}, 3$             |
| Ring of Stars                       | $\frac{3}{2}$                |
| Clique                              | $-(N - 1)$                   |
| Conjoined Cliques                   | $N^2$                        |
| Star of Cliques                     | $N$                          |
| Hierarchy of Cliques                | $N$                          |
| Ring of Cliques                     | $N$                          |
| The Rich Club                       | $-N$                         |
| Conjoined Rich Clubs                | m                            |
| Complete Bipartite                  | Inf                          |
| Conjoined Complete Bipartite Graphs | $2N$                         |

TABLE I  
SUMMARY

| Graph                               | Parameters                                                                                       | Limit/Special case                 | $\left(\frac{b}{c}\right)^*$                                                              |
|-------------------------------------|--------------------------------------------------------------------------------------------------|------------------------------------|-------------------------------------------------------------------------------------------|
| Star                                | $n$ leaf nodes                                                                                   | N/A                                | Inf                                                                                       |
| Extended Star                       | two layers, each $n$ nodes                                                                       | $n \rightarrow \infty$             | $\frac{28}{11} \approx 2.55$                                                              |
| 3-Layer Extended Star               | three layers, each $n$ nodes                                                                     | $n \rightarrow \infty$             | $\frac{106940}{41723} \approx 2.56$                                                       |
| Imperfect Extended Star             | Layer one $n$ nodes, Layer two $n_g$ nodes                                                       | $n_g \ll n$                        | $\frac{34}{89n_g}n \approx \frac{0.38}{n_g}n$                                             |
| Star of Stars                       | $n$ leaf nodes, each connected to $n_d$ nodes                                                    | $n \ll n_d$                        | $\left(2 + \frac{1}{n-1}\right) + \left(\frac{1}{2} + \frac{1}{1-n}\right) \frac{1}{n_d}$ |
| Imperfect Star of Stars             | $n$ leaf nodes, $n_g$ of them connected to $n_d$ nodes                                           | $n_g \ll n \ll n_d$                | $\frac{3}{2} + \frac{1}{2(n_g-1)}$                                                        |
| Two Stars: Hub to Leaf              | Two stars, each with $n$ leaf nodes                                                              | $n \rightarrow \infty$             | $\frac{5}{2}$                                                                             |
| Two Stars: Leaf to Leaf             | Two stars, each with $n$ leaf nodes                                                              | $n \rightarrow \infty$             | 3                                                                                         |
| Ring of Stars                       | $L$ stars, each with $n$ leaf nodes                                                              | $n \rightarrow \infty$             | $\frac{3L-1}{2L-2}$                                                                       |
| Clique                              | $n$ nodes                                                                                        | N/A                                | $-(n-1)$                                                                                  |
| Conjoined Cliques                   | two cliques, each with $n$ nodes                                                                 | $n \rightarrow \infty$             | $n^2$                                                                                     |
| Star of Cliques                     | $m$ cliques, each with $n$ nodes                                                                 | $n \rightarrow \infty$             | $\left(\frac{m}{m-2}\right)n - \frac{(m+8)(m-1)}{(m-2)^2}$                                |
| Connecting Two Cliques via a Star   | two cliques of size $n$ connecting via a star of size $m$                                        | $m = n, n \rightarrow \infty$      | $n - \frac{1}{2}$                                                                         |
| Hierarchy of Cliques                | $q^2$ cliques of size $n$ , at the bottom layer, connected to the base node via $q$ middle nodes | $n \rightarrow \infty$             | $\left[\frac{q^2(2q^2+q+1)}{q^2(2q^2+q+3)-6q-4}\right]n$                                  |
| Ring of Cliques                     | $L$ cliques of size $n$                                                                          | $n \rightarrow \infty$             | $\left(\frac{L}{L-2}\right)n - \frac{(L+1)^2-5}{(L-2)^2}$                                 |
| The Rich Club                       | $N$ hubs and $N-m$ leaves                                                                        | $N \rightarrow \infty$             | $-\frac{2N}{3} \frac{2m-1}{m-1} + \frac{1}{18} \left[8m+39 + \frac{20}{m-1}\right]$       |
| Conjoined Rich Clubs                | two rich clubs, each with $N_c$ core and $N_p$ peripheral nodes                                  | $N_p \rightarrow \infty$           | $4N_c - \frac{3}{2}$                                                                      |
| Complete Bipartite                  | two subsets of nodes with sizes $n_x$ and $n_y$                                                  | N/A                                | Inf                                                                                       |
| Conjoined Complete Bipartite Graphs | two identical complete bipartite graphs with sizes $n_x$ and $n_y$                               | $n_x = n_y = n \rightarrow \infty$ | $2n-1$                                                                                    |
